# Supplementary material for: Crystallography-driven molecularization of a two-dimensional spin-$3/2$ magnet
Source: arXiv:2602.22005 source file (2026-06-10)
Supplement: Supplementary file 1 [file supplement.pdf]

# Supplementary material to Crystallography-driven molecularization of a two-dimensional spin-3/2 magnet

Hari Borutta,<sup>1</sup> Tobias Müller,<sup>2</sup> Ronny Thomale,<sup>2,1</sup> Harald O. Jeschke,<sup>3,1</sup> and Yasir Iqbal<sup>1</sup>

<sup>1</sup>*Department of Physics, Indian Institute of Technology Madras, Chennai 600036, India*

<sup>2</sup>*Institut für Theoretische Physik und Astrophysik and Würzburg-Dresden Cluster of Excellence ct.qmat, Julius-Maximilians-Universität Würzburg, Am Hubland, Campus Süd, Würzburg 97074, Germany*

<sup>3</sup>*Research Institute for Interdisciplinary Science, Okayama University, Okayama 700-8530, Japan*

(Dated: February 25, 2026)

## SUPPLEMENTARY NOTE 1: CRYSTAL STRUCTURE AND DENSITY FUNCTIONAL THEORY CALCULATIONS

The microscopic origin of the anomalous magnetic behavior of  $\text{Na}_2\text{Mn}_3\text{O}_7$  lies not simply in geometric frustration, but in the low crystallographic symmetry of the material. The triclinic crystal structure hosts three symmetry-inequivalent  $\text{Mn}^{4+}$  sites, which partition the maple-leaf lattice into distinct exchange pathways already at the nearest-neighbor level. This crystallographic inequivalence is the key ingredient that generates a strong hierarchy of exchange interactions, reorganizing the low-energy degrees of freedom from individual spins into emergent hexagonal units. To quantify this hierarchy and establish a realistic microscopic Hamiltonian, we employ density-functional-theory-based (DFT) energy mapping, which provides a direct and unbiased determination of the relevant exchange couplings.

The full crystal structure of  $\text{Na}_2\text{Mn}_3\text{O}_7$  has been determined by Chang and Jansen in 1985 [1], by Raekelboom *et al.* in 2001 [2], and by Song *et al.* in 2019 [3]. Total energy calculated with the all electron full potential local orbital (FPLO) [4] and generalized gradient approximation (GGA) [5] is best for the oldest, single crystal X-ray diffraction (XRD) structure. The 2019 XRD structure is 0.2 eV/f.u. higher, the 2019 neutron diffraction structure is 0.9 eV/f.u. higher, and the 2001 structure is 1.9 eV/f.u. higher in energy. For this reason, we use the single-crystal XRD structure determined by Chang and Jansen [1] in this study. We emphasize that, within our tests, the qualitative exchange hierarchy  $J_{1,2,3} \gg |J_{4-9}|$  is a robust feature of the material and does not rely on fine structural details, although the weaker couplings naturally exhibit a stronger structure dependence.

In Fig. 1 of the main text, we show the result of the DFT energy mapping based on a  $\sqrt{3} \times 1 \times \sqrt{3}$  supercell of  $\text{Na}_2\text{Mn}_3\text{O}_7$ . Due to the low symmetry of the crystal (triclinic space group  $P\bar{1}$ ) with three symmetry inequivalent  $\text{Mn}^{4+}$  ( $S = 3/2$ ) sites, the maple leaf lattice is defined by nine distinct "nearest neighbor" bonds, nine "second nearest neighbors" (three of them inside the hexagon) and nine "third nearest neighbors" (again three of them inside the hexagon). These neighbors are all identified by Mn-Mn distance (measured in the structure of Ref. 1) in Table I of the main text. The energy mapping results are shown for different values of the onsite interaction

strength  $U$  in Fig. 1(a) of the main text, and information about the overall energy scale of the material is necessary for choosing the relevant  $U$  value. We rely on Ref. 6 that gives a value of  $\theta_{\text{CW}} = -152$  K for the Curie-Weiss temperature, based on a fit to the magnetic susceptibility  $\chi(T)$ . The resulting Heisenberg Hamiltonian, specified fully in Table I of the main text in spite of its complexity provides a clear picture for the magnetism of  $\text{Na}_2\text{Mn}_3\text{O}_7$ . The resulting exchange pattern exhibits a pronounced hierarchy: (i) three dominant antiferromagnetic couplings ( $J_1$ – $J_3$ ) forming strongly correlated hexagons, (ii) six sizable ferromagnetic interactions ( $J_4$ – $J_9$ ) coupling these hexagons, and (iii) weaker but non-negligible second- and third-neighbor interactions that further frustrate magnetic ordering. Weak interlayer couplings and longer-range in-plane interactions, which are at least an order of magnitude smaller than  $J_h$ , are neglected in the effective model and are not expected to qualitatively alter the cluster-dominated physics discussed here.

The pronounced hierarchy of exchange couplings can be traced to the low-symmetry superexchange geometry of the Mn–O network. The dominant intra-hexagon bonds are mediated by two shared oxygen ligands, enhancing antiferromagnetic superexchange, whereas the weaker inter-hexagon bonds involve single-oxygen bridges and reduced hybridization. While simple Goodenough–Kanamori considerations provide qualitative guidance, detailed microscopic analysis in low-symmetry environments is subtle and can be misleading if applied heuristically. The exchange hierarchy reported in Table I of the main text is therefore established directly via *ab initio* energy mapping and is robust against small variations of computational parameters.

## SUPPLEMENTARY NOTE 2: MICROSCOPIC (SUPEREXCHANGE) ORIGIN OF THE EXCHANGE HIERARCHY

The hierarchy of exchange couplings obtained from total-energy mapping can be understood microscopically from the geometry of the Mn–O–Mn superexchange pathways.  $\text{Mn}^{4+}$  ions in  $\text{Na}_2\text{Mn}_3\text{O}_7$  have a  $3d^3$  ( $t_{2g}^3$ ,  $S = 3/2$ ) configuration, for which the magnitude of isotropic exchange is controlled primarily by the strength of Mn–O hybridization and the number and geometry of bridging ligands, in the spirit of the Goodenough–Kanamori–

TABLE S1. Local superexchange geometry for the nine nearest-neighbor Mn–Mn exchange paths. For each bond class  $J_i$  (identified using the same nearest-neighbor definition as in Table I, we list the Mn–Mn distance  $d_{\text{MnMn}}$ , the number of shared (bridging) oxygens  $n_{\text{O}}^{\text{bridge}}$ , the mean Mn–O distance  $\langle d_{\text{MnO}} \rangle$  over the shared oxygens, and the corresponding Mn–O–Mn bond-angle range. While all nine bonds involve bent Mn–O–Mn geometries in a near-90° window, the dominant intra-hexagon couplings  $J_{1,2,3}$  are distinguished by double-oxygen bridges and systematically shorter Mn–O distances compared to the weaker couplings  $J_{4-9}$ , consistent with an enhanced antiferromagnetic superexchange scale.

| $J_i$ | $d_{\text{MnMn}}$ (Å) | $n_{\text{O}}^{\text{bridge}}$ | $\langle d_{\text{MnO}} \rangle$ (Å) | $\angle \text{Mn–O–Mn}$ (deg) |
|-------|-----------------------|--------------------------------|--------------------------------------|-------------------------------|
| $J_1$ | 2.7887                | 2                              | 1.882                                | 93.37–97.95                   |
| $J_2$ | 2.8003                | 2                              | 1.871                                | 95.26–98.64                   |
| $J_3$ | 2.8050                | 2                              | 1.891                                | 93.35–98.33                   |
| $J_4$ | 2.9305                | 1                              | 1.96                                 | $\sim 97$                     |
| $J_5$ | 2.9348                | 1                              | 1.97                                 | $\sim 96$                     |
| $J_6$ | 2.9435                | 1                              | 1.98                                 | $\sim 96$                     |
| $J_7$ | 2.9505                | 1                              | 1.97                                 | $\sim 97$                     |
| $J_8$ | 2.9550                | 1                              | 1.97                                 | $\sim 97$                     |
| $J_9$ | 2.9606                | 1                              | 1.97                                 | $\sim 97$                     |

Anderson rules.

Using the same definition of the nearest-neighbor manifold as in the energy-mapping procedure—namely, the nine shortest Mn–Mn bonds per Mn site—we analyzed the local exchange geometry for each bond class [Table S1]. We find that the shortest Mn–Mn links, which form the hexagonal backbone of the Mn sublattice and correspond to the dominant couplings  $J_{1,2,3}$ , are mediated by two shared oxygen ligands [Table S1], with bent Mn–O–Mn bond angles in the range  $\sim 93^\circ$ – $99^\circ$ . These double-oxygen bridges enhance the effective Mn–O hybridization and thus maximize the antiferromagnetic superexchange scale.

In contrast, the remaining bonds within the nine-nearest-neighbor manifold involve weaker superexchange pathways characterized by single oxygen bridges, longer Mn–O distances, and reduced effective hybridization, as summarized in Table S1. For such geometries, the antiferromagnetic hopping channel is suppressed, and competing virtual processes—including Hund’s-rule-assisted contributions—become comparably important, resulting in significantly weaker exchange interactions.

We emphasize that the relevant mechanism is oxygen-mediated superexchange rather than direct  $d$ – $d$  overlap. The strength of the interaction is therefore controlled not only by the Mn–Mn distance, but crucially by the Mn–O bond lengths, bond angles, and the number of bridging ligands. In the present structure, three Mn–Mn bonds are connected by double Mn–O–Mn bridges with comparatively short Mn–O distances, while the remaining six bonds are mediated by single bridges with longer Mn–O separations. This structural dichotomy naturally partitions the exchange network into two groups and provides a microscopic explanation for the hierarchy  $J_{1,2,3} \gg |J_{4-9}|$  obtained from total-energy mapping.

Even modest ( $\sim 3$ – $5\%$ ) reductions in the Mn–O distance between the double-oxygen-bridged hexagon bonds and the remaining links can translate into substantial differences in effective hopping amplitudes and hence large variations in the resulting exchange couplings, consistent

with the hierarchy obtained from the *ab initio* calculations. Importantly, this hierarchy is not the result of fine tuning but follows directly from the low-symmetry crystallographic structure.

It is worth emphasizing the limitations of heuristic superexchange arguments in low-symmetry, multi-path systems such as  $\text{Na}_2\text{Mn}_3\text{O}_7$ . As illustrated by the extended discussion in Ref. [7], plausible-looking Goodenough–Kanamori–Anderson-type considerations can sometimes lead to mutually contradictory or even incorrect conclusions when applied in isolation. In the present case, the commonly invoked Mn–Mn distance argument, adopted from Ref. [8] in subsequent experimental analyses, fails to account for either the sign or the magnitude of the dominant exchange interactions. Instead, the leading antiferromagnetic couplings correlate systematically with the number and geometry of bridging oxygen ligands, with two-oxygen exchange paths consistently dominating over single-oxygen bridges.

Importantly, however, we do not regard this observation as a universal rule. Rather, it serves only as a qualitative rationalization of the exchange hierarchy obtained from *ab initio* energy mapping. The central and robust result of our analysis is the exchange hierarchy itself, which follows directly from the electronic structure calculations and does not depend on assuming the transferability of any particular superexchange heuristic to other materials or lattice geometries.

We refer to this reorganization of the magnetic degrees of freedom into strongly correlated hexagonal units as *molecularization* of the magnet: a regime in which local cluster physics dominates thermodynamics, while inter-cluster coherence is governed by weaker, frustrated couplings.

In summary, the microscopic Heisenberg Hamiltonian derived from DFT reveals a clear physical picture: strongly antiferromagnetic hexagonal building blocks are embedded in a network of competing ferromagnetic interactions, producing frustration already at the classical level. This explains both the absence of conventional

magnetic order and the dominance of short-range correlations in  $\text{Na}_2\text{Mn}_3\text{O}_7$ .

### SUPPLEMENTARY NOTE 3: LATTICE DEFINITION

We use the following convention for the primitive lattice and basis vectors for a single Mn-layer in  $\text{Na}_2\text{Mn}_3\text{O}_7$  in units of Angstrom:

$$\mathbf{a}_1 = (-3.7617292, -6.5719928, 0), \quad (\text{S1a})$$

$$\mathbf{a}_2 = (7.548, 0, 0), \quad (\text{S1b})$$

$$\mathbf{a}_3 = (0.0630616, 0.4838087, 11.1473178); \quad (\text{S1c})$$

$$\mathbf{b}_1 = (-0.2314105, -1.4489934, 0.0105900), \quad (\text{S2a})$$

$$\mathbf{b}_2 = (0.2314105, 1.4489934, -0.0105900), \quad (\text{S2b})$$

$$\mathbf{b}_3 = (2.3987910, -0.52321930, -0.0323272), \quad (\text{S2c})$$

$$\mathbf{b}_4 = (-2.3987910, 0.52321930, 0.0323272), \quad (\text{S2d})$$

$$\mathbf{b}_5 = (3.0371082, 2.3617041, 0.0089179), \quad (\text{S2e})$$

$$\mathbf{b}_6 = (-3.0371082, -2.3617041, -0.0089179). \quad (\text{S2f})$$

In this convention, a second layer is present in the unit cell, shifted by  $0.5\mathbf{a}_1 + 0.5\mathbf{a}_2 + 0.5\mathbf{a}_3$  with respect to the one given.

### SUPPLEMENTARY NOTE 4: CLASSICAL GROUND STATE: LUTTINGER-TISZA ANALYSIS

Before addressing the quantum problem, it is instructive to analyze the classical ground state of the microscopic Heisenberg Hamiltonian. Beyond providing a reference point, this analysis clarifies whether the pronounced hierarchy of exchange couplings stabilizes a robust classical order or instead leads to a fragile ordering tendency that is highly susceptible to fluctuations. As we show below, the latter scenario applies: while a unique classical ordering wavevector is selected, the corresponding energy scale is exceedingly small, placing the system close to the boundary between conventional long-range order and frustration-induced melting.

### A. Luttinger–Tisza formulation

We treat the  $\text{Mn}^{4+}$  moments as classical spins of fixed length  $|\mathbf{S}_i| = S$  and consider the classical Hamiltonian

$$H_{\text{cl}} = \sum_{i,j} J_{ij} \mathbf{S}_i \cdot \mathbf{S}_j. \quad (\text{S3})$$

To determine the dominant ordering tendencies, we employ the Luttinger–Tisza (LT) method, which relaxes the local hard-spin constraint to a global one and reduces the problem to minimizing the lowest eigenvalue of the Fourier-transformed exchange matrix  $\mathcal{J}_{\alpha\beta}(\mathbf{k})$ , where  $\alpha, \beta = 1, \dots, 6$  label the sublattices of the maple-leaf unit cell. All classical energies are quoted in Kelvin units, consistent with the exchange parameters in Table I of the main text. We use an extension of the method, which allows us to treat lattices with multiple sublattices exactly [9]. To achieve this, a dressed interaction matrix

$$\tilde{\mathcal{J}}_{\alpha\beta}(\mathbf{k}, \lambda) = \mathcal{J}_{\alpha\beta}(\mathbf{k}) + \lambda_{\alpha} \delta_{\alpha\beta}, \quad \sum_{\alpha} \lambda_{\alpha} = 0 \quad (\text{S4})$$

is introduced. If the hard-spin constraint is fulfilled, this does not change the energies of the system, but gives a handle on tuning the relative spin length of the sublattices for the relaxed version. In the case of a ground state determined by a single  $\mathbf{q}$ -vector, the configuration is found by maximizing w.r.t  $\lambda$ , the minimal eigenvalue of  $\tilde{\mathcal{J}}_{\alpha\beta}(\mathbf{k}, \lambda)$ , within the first Brillouin zone.

Following the equivalence of basis sites under inversion and guided by the eigenvector-structure of  $\tilde{\mathcal{J}}_{\alpha\beta}(\mathbf{k}, \lambda = \mathbf{0})$ , we choose

$$\lambda_1 = \lambda_2 = a \quad (\text{S5})$$

$$\lambda_3 = \lambda_4 = -a - b \quad (\text{S6})$$

$$\lambda_5 = \lambda_6 = b \quad (\text{S7})$$

as an *Ansatz* for the parameters.

Diagonalizing  $\tilde{\mathcal{J}}_{\alpha\beta}(\mathbf{k}, \lambda)$  throughout the Brillouin zone yields a unique global minimum at an incommensurate wavevector

$$\mathbf{k}_0 \simeq (0.500290721994559, 0.04252249458547225, 0) \text{ \AA}^{-1}. \quad (\text{S8})$$

for  $a = 9.54$ ,  $b = -10.24$  with corresponding minimal eigenvalue

$$\lambda_{\min}(\mathbf{k}_0) = -206.415 \text{ K}. \quad (\text{S9})$$

This implies a classical energy per spin,

$$E_{\text{LT}} = \frac{1}{2} \lambda_{\min}(\mathbf{k}_0) = -103.208 \text{ K}. \quad (\text{S10})$$

The ordering wavevector lies close to one of the  $K$ -points of the Brillouin zone, but is not locked onto it, indicating that the ordering is not symmetry-enforced but instead arises from a subtle balance between the dominant antiferromagnetic couplings within the hexagonal motifs and weaker, frustrated inter-hexagon interactions.

## B. Local structure of the LT minimum

To assess the rigidity of this ordering tendency, we examine the curvature of the LT spectrum in the vicinity of  $\mathbf{k}_0$ . A fine momentum-space scan yields the Hessian

$$H_{ij} = \partial_{k_i} \partial_{k_j} \lambda_{\min}(\mathbf{k})|_{\mathbf{k}_0} = \begin{pmatrix} 371.161 & 75.406 \\ 75.406 & 152.402 \end{pmatrix}, \quad (\text{S11})$$

with eigenvalues 394.635 and 128.929. While the minimum is clearly isolated, the pronounced anisotropy of the curvature reflects a relatively shallow energy landscape, particularly along one momentum direction. This already signals a weakly stabilized classical order.

The corresponding LT eigenvector at  $\mathbf{k}_0$ ,

$$v_0 = (v_1, \dots, v_6), \quad (\text{S12})$$

is complex with its phases defining fixed sublattice offsets

$$\phi_\alpha = \arg(v_\alpha). \quad (\text{S13})$$

These indicate an almost perfect antiferromagnetic alignment of spins around a hexagon, canted only by a maximum of  $0.02\pi$  from the perfect antiparallel alignment.

## C. Physical state

The classical ground state may therefore be characterized as a weakly stabilized, incommensurate spiral with slowly varying relative orientations between strongly approximately antiferromagnetically correlated hexagons. The dominant couplings  $J_{1-3}$  enforce nearly collinear antiferromagnetic correlations within each hexagon, while weaker and partly frustrated inter-hexagon couplings select a unique relative phase only at a very small energy scale. Although the inter-hexagon couplings are substantially weaker than the dominant intra-hexagon exchanges, they remain essential for selecting the incommensurate ordering wavevector and for shaping the momentum-space structure of correlations. Thus, the incommensurate nature of the ordering wave-vector reflects the competition between nearly isolated hexagonal units and the frustrated network of weak inter-hexagon couplings, which cannot be simultaneously satisfied at any commensurate momentum.

From a broader perspective, the system lies close to the boundary between order-by-disorder and melting-by-frustration scenarios. Although a specific ordering wavevector is selected at the classical level, the associated selection energy is exceedingly small and the energy landscape is shallow and anisotropic. As a result, the system is highly susceptible to both thermal and quantum fluctuations.

This conclusion provides a natural bridge to the results presented in the following section. Classical Monte Carlo (cMC) simulations capture the dominant short-range correlations and reveal only incipient ordering at the lowest temperatures, while the pseudofermion functional renormalization group (pf-FRG) demonstrates that quantum fluctuations melt this fragile classical order entirely. In this sense, the LT analysis already anticipates the central message of this work:  $\text{Na}_2\text{Mn}_3\text{O}_7$  resides in a regime where a crystallography-induced exchange hierarchy produces strong local correlations but leaves long-range order only marginally stable, rendering it exceptionally sensitive to fluctuation effects. Thus, the suppression of long-range order is not driven by an extensive classical degeneracy, but rather by the extremely small energy scale associated with an otherwise uniquely selected incommensurate spiral.

Taken together, the classical analysis identifies a uniquely selected but extremely weak incommensurate spiral, whose fragility already anticipates the absence of long-range order once thermal or quantum fluctuations are included. From this viewpoint, the LT analysis fixes the dominant momentum-space structure of correlations, cMC quantifies their thermal evolution, and the pf-FRG establishes their survival as short-range quantum correlations without symmetry breaking.

## SUPPLEMENTARY NOTE 5: LOW-TEMPERATURE CMC SPIN CONFIGURATION AND PF-FRG FLOWS

As stated in the main text, the cMC calculations result in the development of magnetic order, at least for systems of finite sizes. Fig. S1 shows the magnetic unit cell in a portion of the  $40 \times 40$  cMC spin configuration at a temperature of 0.001K. This magnetic ordering is consistent with the ordering vector determined using the LT method. In a simulation with periodic boundary conditions, only ordering vectors respecting these are possible to select, with the ordering being the closest one to the actual incommensurate wave-vector. At any rate, the true nature of the ground state is better revealed by incorporating quantum fluctuations through the pf-FRG technique.

The disordered nature of the original ground state can be inferred from the pf-FRG flow of the maximum value of the structure factor and its second derivative for various system sizes (see Fig. S2). The flow curves for these different system sizes overlap on top of each other, and the smooth monotonic increase with decrease in the cut-off value implies that there is no conventional long-range magnetic ordering.

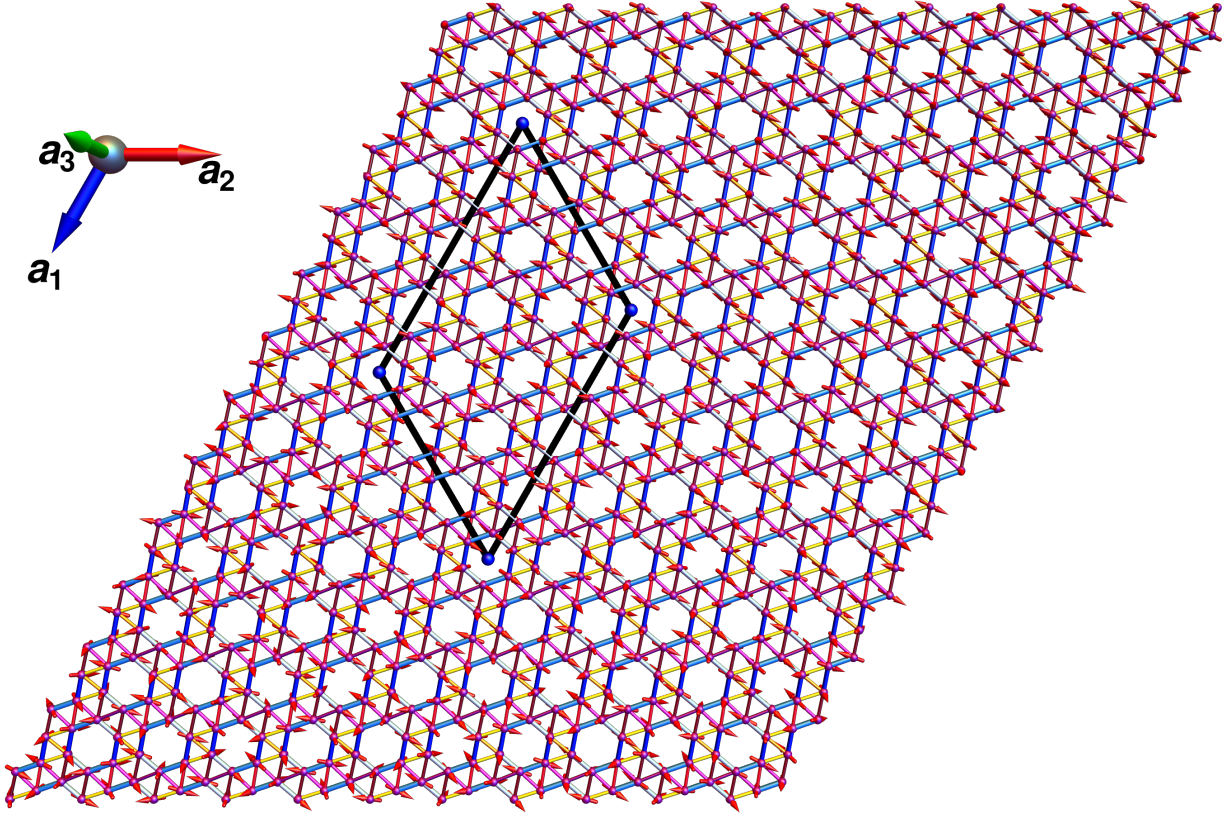

FIG. S1. Representative low-temperature cMC spin configuration illustrating the incipient ordering tendency at finite size. Shown is a portion of a  $40 \times 40$  system at  $T = 0.001$  K; arrows indicate spin orientations, and the repeating pattern highlights the emergent magnetic unit cell produced by the shallow classical energy landscape.

- 
- [1] F. M. Chang and M. Jansen, Darstellung und Kristallstruktur von  $\text{Na}_2\text{Mn}_3\text{O}_7$ , *Z. Anorg. Allg. Chem.* **531**, 177 (1985).
  - [2] E. A. Raelboom, A. L. Hector, J. Owen, G. Vitins, and M. T. Weller, Syntheses, structures, and preliminary electrochemistry of the layered lithium and sodium manganese(IV) oxides,  $\text{A}_2\text{Mn}_3\text{O}_7$ , *Chem. Mater.* **13**, 4618 (2001).
  - [3] B. Song, M. Tang, E. Hu, O. J. Borkiewicz, K. M. Wiaderek, Y. Zhang, N. D. Phillip, X. Liu, Z. Shadike, C. Li, L. Song, Y.-Y. Hu, M. Chi, G. M. Veith, X.-Q. Yang, J. Liu, J. Nanda, K. Page, and A. Huq, Understanding the low-voltage hysteresis of anionic redox in  $\text{Na}_2\text{Mn}_3\text{O}_7$ , *Chem. Mater.* **31**, 3756 (2019).
  - [4] K. Koepnik and H. Eschrig, Full-potential nonorthogonal local-orbital minimum-basis band-structure scheme, *Phys. Rev. B* **59**, 1743 (1999).
  - [5] J. P. Perdew, K. Burke, and M. Ernzerhof, Generalized gradient approximation made simple, *Phys. Rev. Lett.* **77**, 3865 (1996).
  - [6] C. Venkatesh, B. Bandyopadhyay, A. Midya, K. Mahalingam, V. Ganesan, and P. Mandal, Magnetic properties of the one-dimensional  $S = \frac{3}{2}$  Heisenberg antiferromagnetic spin-chain compound  $\text{Na}_2\text{Mn}_3\text{O}_7$ , *Phys. Rev. B* **101**, 184429 (2020).
  - [7] B. Saha, A. K. Bera, S. M. Yusuf, and A. Hoser, Two-dimensional short-range spin-spin correlations in the layered spin- $\frac{3}{2}$  maple leaf lattice antiferromagnet  $\text{Na}_2\text{Mn}_3\text{O}_7$  with crystal stacking disorder, *Phys. Rev. B* **107**, 064419 (2023).
  - [8] Y. Haraguchi, A. Matsuo, K. Kindo, and Z. Hiroi, Frustrated magnetism of the maple-leaf-lattice antiferromagnet  $\text{MgMn}_3\text{O}_7 \cdot 3\text{H}_2\text{O}$ , *Phys. Rev. B* **98**, 064412 (2018).
  - [9] H.-J. Schmidt and J. Richter, Classical ground states of spin lattices, *J. Phys. A: Math. Theor.* **55**, 465005 (2022).

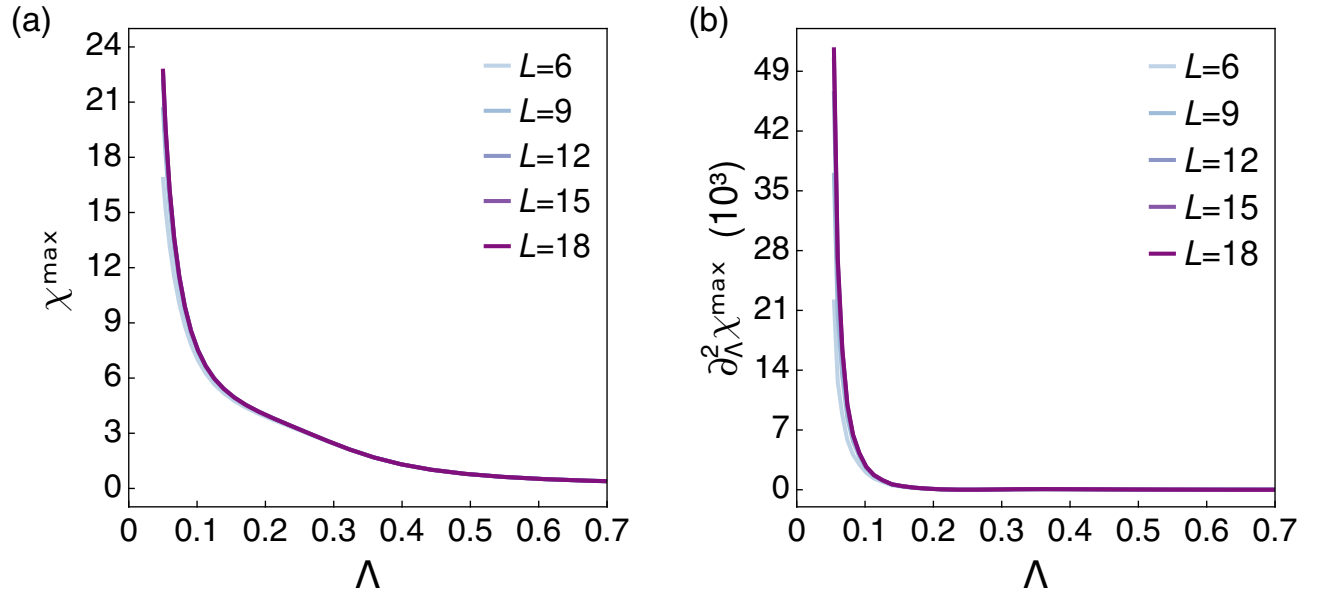

FIG. S2. pf-FRG flows demonstrating the absence of a dipolar magnetic ordering instability. (a) Flow of the maximum of the static structure factor,  $\chi^{\max}(\Lambda) = \max_{\mathbf{k}} \chi_{\Lambda}^{zz}(\mathbf{k})$ , as the infrared cutoff  $\Lambda$  is lowered, shown for several truncation ranges / system sizes. (b) Corresponding second derivative  $d^2\chi^{\max}/d\Lambda^2$ . The overlap of curves for different system sizes and the smooth, monotonic evolution without a size-enhancing nonmonotonic feature indicate no pf-FRG flow breakdown and hence no conventional long-range dipolar order.
